# Supplementary material for: Accelerating Fully Homomorphic Encryption by Bridging Modular and Bit-Level Arithmetic
Source: arXiv:2204.12201 source file (2023-01-13)
Supplement: Supplementary file 1 [file A-appendix.tex]

\vspace{-0.8cm}
\section*{Appendix}
\vspace{-0.2cm}
We include in this appendix the codes referent to the benchmarks used in \ref{ss:benchmarks}. The codes presented feature \secint, but the code using \secuint\ is similar.

\vspace{-0.1cm}
\begin{figure}[h]

%\scriptsize
% \vbox to 600pt {
\noindent\begin{minipage}{.50\textwidth}
\begin{lstlisting}[language=C++,
caption={Private Keyword Search using bit-level arithmetic.},
style=mystyle, label=list:pks_bit,
%framexrightmargin=-37pt,
% xleftmargin=0.4cm,
% xrightmargin=-0.12\linewidth,
% linewidth=0.88\linewidth
]
template <int S> SecureInt<S>
pks(vector<SecureInt<S>> v, SecureInt<S> k)
{
    vector<SecureInt<S>> r;
    for (size_t i=0; i < v.size(); i++)
    {
        auto eq = i == k;
        auto sel = eq * v[i];
        r.push_back(sel);
    }
    return sum(r);
}
\end{lstlisting}
\end{minipage}
% \vspace{\lstbspace}

% }
\end{figure}

\vspace{-1.3cm}
\begin{figure}[h]
%\scriptsize
\noindent\begin{minipage}{.50\textwidth}
\begin{lstlisting}[language=C++,
caption={Private Keyword Search with bridging.},
style=mystyle, label=list:pks_bridge,
%framexrightmargin=-37pt,
% xleftmargin=0.4cm,
% xrightmargin=-0.12\linewidth,
% linewidth=0.88\linewidth
]
template <int S> SecureMod
pks(vector<SecureInt<S>> v, SecureInt<S> k)
{
    vector<SecureMod> r;
    for (size_t i=0; i < v.size(); i++)
    {
        auto eq = i == k;
        auto sel = eq * SecureMod(v[i]);
        r.push_back(sel);
    }
    return sum(r);
}
\end{lstlisting}
\end{minipage}
% \vspace{\lstbspace}
\end{figure}

% \begin{figure}[t]
% %\scriptsize
% \noindent\begin{minipage}{.45\textwidth}
% \begin{lstlisting}[language=C++,
% caption={Private Keyword Search with bridging.},
% style=mystyle, label=list:pks_bit,
% %framexrightmargin=-37pt,
% % xleftmargin=0.4cm,
% % xrightmargin=-0.12\linewidth,
% % linewidth=0.88\linewidth
% ]
% template <int S> SecureMod
% pks(vector<SecureInt<S>> v, SecureInt<S> k)
% {
%     vector<SecureMod> r;
%     for (size_t i=0; i < v.size(); i++)
%     {
%         auto eq = i == k;
%         auto sel = eq * SecureMod(v[i]);
%         r.push_back(sel);
%     }
%     return sum(r);
% }
% \end{lstlisting}
% \end{minipage}
% % \vspace{\lstbspace}
% \end{figure}

\begin{figure}[t]
%\scriptsize
\begin{minipage}{\linewidth}
\begin{lstlisting}[language=C++,
caption={Logistic regression with data filtering using bit-level arithmetic.},
style=mystyle, label=list:log_bit,
%framexrightmargin=-37pt,
% xleftmargin=0.4cm,
% xrightmargin=-0.12\linewidth,
% linewidth=0.88\linewidth
]
template <class T> vector<vector<T>>
appendCol(vector<vector<T>> m, T value)
{
  for (auto & v : m) v.push_back(value);
  return m;
}

template <int S>
vector<vector<SecureInt<S>>>
filter(vector<vector<SecureInt<S>>> m,
  SecureInt<S> threshold, vector<int> pos)
{
  for (auto & idx : pos)
  {
    for (auto & v : m)
    {
      auto cond = v[idx] > threshold;
      v[idx] = cond * threshold
            + !cond * v[idx];
    }
  }
  return m;
}

template <int S>
vector<vector<SecureInt<S>>>
mm(vector<vector<SecureInt<S>>> a,
  vector<vector<SecureInt<S>>> b)
{
  auto n = a.size();
  auto m = b.size();
  auto p = b[0].size();
  vector<vector<SecureInt<S>>> c(n);
  for (size_t i=0; i<n; i++)
  {
    for (size_t j=0; j<p; j++)
    {
      vector<SecureInt<S>> t;
      for (size_t k=0; k<m; k++)
        t.push_back(a[i][k] * b[k][j]);
      c[i].push_back(sum(t));
    }
  }
  return c;
}

template <int S>
vector<vector<SecureInt<S>>>
logreg(vector<vector<SecureInt<S>>> inputs,
  vector<vector<SecureInt<S>>> weights,
  SecureInt<S> threshold, vector<int> pos)
{
  SecureInt<S> one = _1_E;
  filter(inputs, threshold, pos);
  auto inputsU = convert(inputs, one);
  appendCol(inputsU, one);
  return mm(inputsU, weights);
}
\end{lstlisting}
\end{minipage}
% \vspace{\lstbspace}
\end{figure}

\begin{figure}[b]
%\scriptsize
\begin{minipage}{\linewidth}
\begin{lstlisting}[language=C++,
caption={Logistic regression with data filtering using bridging.},
style=mystyle, label=list:log_bridge,
%framexrightmargin=-37pt,
% xleftmargin=0.4cm,
% xrightmargin=-0.12\linewidth,
% linewidth=0.88\linewidth
]
template <class T> vector<vector<T>>
appendCol(vector<vector<T>> m, T value)
{
  for (auto & v : m) v.push_back(value);
  return m;
}

template <int S>
vector<vector<SecureInt<S>>>
filter(vector<vector<SecureInt<S>>> m,
  SecureInt<S> threshold, vector<int> pos)
{
  for (auto & idx : pos)
  {
    for (auto & v : m)
    {
      auto cond = v[idx] > threshold;
      v[idx] = cond * threshold
            + !cond * v[idx];
    }
  }
  return m;
}


vector<vector<SecureMod>>
mm(vector<vector<SecureMod>> a,
  vector<vector<SecureMod>> b)
{
  auto n = a.size();
  auto m = b.size();
  auto p = b[0].size();
  vector<vector<SecureMod>> c(n);
  for (size_t i=0; i<n; i++)
  {
    for (size_t j=0; j<p; j++)
    {
      vector<SecureMod> t;
      for (size_t k=0; k<m; k++)
        t.push_back(a[i][k] * b[k][j]);
      c[i].push_back(sum(t));
    }
  }
  return c;
}

template <int S>
vector<vector<SecureMod>>
logreg(vector<vector<SecureInt<S>>> inputs,
  vector<vector<SecureMod>> weights,
  SecureInt<S> threshold, vector<int> pos)
{
  SecureMod one = _1_M;
  filter(inputs, threshold, pos);
  auto inputsU = convert(inputs, one);
  appendCol(inputsU, one);
  return mm(inputsU, weights);
}
\end{lstlisting}
\end{minipage}
% \vspace{\lstbspace}
\end{figure}

\begin{figure}[t]
%\scriptsize
\begin{minipage}{\linewidth}
\begin{lstlisting}[language=C++,
caption={Bit-level depth-optimized max function.},
style=mystyle, label=list:max_bit,
%framexrightmargin=-37pt,
% xleftmargin=0.4cm,
% xrightmargin=-0.12\linewidth,
% linewidth=0.88\linewidth
]









template <int S> vector<SecureInt<S>>
indices(vector<SecureInt<S>> v)
{
  int size = v.size();
  vector<SecureInt<S>> idx;
  vector<vector<SecureInt<S>>> m(size);
  for (int i=0; i < size; i++)
  {
    for (int j=i+1; j < size; j++)
    {
      auto cond = v[i] > v[j];
      m[i].push_back(SecureInt<S>(cond));
      m[j].push_back(SecureInt<S>(!cond));
    }
    idx.push_back(product(m[i]));
  }
  return idx;
}

template <int S> SecureInt<S>
select(vector<SecureInt<S>> idx,
  vector<SecureInt<S>> v)
{
  int size = v.size();
  vector<SecureInt<S>> r;
  for (int i=0; i < size; i++)
    r.push_back(idx[i] * v[i]);
  return sum(r);
}

template <int S> SecureInt<S>
max(vector<SecureInt<S>> v)
{
  return select(indices(v), v);
}

\end{lstlisting}
\end{minipage}
% \vspace{\lstbspace}
\end{figure}

\begin{figure}[t]
%\scriptsize
\begin{minipage}{\linewidth}
\begin{lstlisting}[language=C++,
caption={The multiplexer function using bit-level arithmetic.},
style=mystyle, label=list:mux_bit,
%framexrightmargin=-37pt,
% xleftmargin=0.4cm,
% xrightmargin=-0.12\linewidth,
% linewidth=0.88\linewidth
]
template <int S> SecureInt<S>
mux(SecureInt<S> input, SecureInt<S> item,
    SecureInt<S> t, SecureInt<S> f)
{
    auto cond = input == item;
    return cond * t
        + !cond * f;
}
\end{lstlisting}
\end{minipage}
% \vspace{\lstbspace}
\end{figure}

\begin{figure}[t]
%\scriptsize
\begin{minipage}{\linewidth}
\begin{lstlisting}[language=C++,
caption={Depth optimized max function with bridging.},
style=mystyle, label=list:max_bridge,
%framexrightmargin=-37pt,
% xleftmargin=0.4cm,
% xrightmargin=-0.12\linewidth,
% linewidth=0.88\linewidth
]
template <class T> vector<SecureMod>
convert(vector<T> v)
{
    vector<SecureMod> u;
    for (auto & e : v)
        u.push_back(SecureMod(e));
    return u;
}

template <int S> vector<SecureMod>
indices(vector<SecureInt<S>> v)
{
  int size = v.size();
  vector<SecureMod> idx;
  vector<vector<SecureMod>> m(size);
  for (int i=0; i < size; i++)
  {
    for (int j=i+1; j < size; j++)
    {
      auto cond = v[i] > v[j];
      m[i].push_back(SecureMod(cond));
      m[j].push_back(SecureMod(!cond));
    }
    idx.push_back(product(m[i]));
  }
  return idx;
}

SecureMod
select(vector<SecureMod> idx,
    vector<SecureMod> v)
{
  int size = v.size();
  vector<SecureMod> r;
  for (int i=0; i < size; i++)
    r.push_back(idx[i] * v[i]);
  return sum(r);
}

template <int S> SecureMod
max(vector<SecureInt<S>> v)
{
  return select(indices(v), convert(v));
}
\end{lstlisting}
\end{minipage}
% \vspace{\lstbspace}
\end{figure}

\begin{figure}[t]
%\scriptsize
\begin{minipage}{\linewidth}
\begin{lstlisting}[language=C++,
caption={The multiplexer function with bridging.},
style=mystyle, label=list:mux_bridge,
%framexrightmargin=-37pt,
% xleftmargin=0.4cm,
% xrightmargin=-0.12\linewidth,
% linewidth=0.88\linewidth
]
template <int S> SecureMod
mux(SecureInt<S> input, SecureInt<S> item,
    SecureInt<S> t, SecureInt<S> f)
{
    auto cond = input == item;
    return cond * SecureMod(t)
        + !cond * SecureMod(f);
}
\end{lstlisting}
\end{minipage}
% \vspace{\lstbspace}
\end{figure}

\begin{figure}[t]
%\scriptsize
\begin{minipage}{\linewidth}
\begin{lstlisting}[language=C++,
caption={Depth-optimized sorting algorithm using bit-level arithmetic.},
style=mystyle, label=list:sor_bit,
%framexrightmargin=-37pt,
% xleftmargin=0.4cm,
% xrightmargin=-0.12\linewidth,
% linewidth=0.88\linewidth
]









template <int S> vector<SecureInt<S>>
indices(vector<SecureInt<S>> v)
{
  int size = v.size();
  vector<SecureInt<S>> idx;
  vector<vector<SecureInt<S>>> m(size);
  for (int i=0; i < size; i++)
  {
    for (int j=i+1; j < size; j++)
    {
      auto cond = v[i] > v[j];
      m[i].push_back(SecureInt<S>(cond));
      m[j].push_back(SecureInt<S>(!cond));
    }
    idx.push_back(sum(m[i]));
  }
  return idx;
}

template <int S> vector<SecureInt<S>>
select(vector<SecureInt<S>> idx,
  vector<SecureInt<S>> v)
{
  int size = v.size();
  vector<SecureInt<S>> r;
  for (int i=0; i < size; i++)
  {
    vector<SecureInt<S>> t;
    for (int j=0; j < size; j++ )
      t.push_back((i == idx[j]) * v[j]);
    r.push_back(sum(t));
  }
  return r;
}

template <int S> vector<SecureInt<S>>
sort(vector<SecureInt<S>> v)
{
  return select(indices(v), v);
}

\end{lstlisting}
\end{minipage}
% \vspace{\lstbspace}
\end{figure}

\begin{figure}[t]
%\scriptsize
\begin{minipage}{\linewidth}
\begin{lstlisting}[language=C++,
caption={Depth-optimized sorting algorithm using bridging.},
style=mystyle, label=list:sor_bridge,
%framexrightmargin=-37pt,
% xleftmargin=0.4cm,
% xrightmargin=-0.12\linewidth,
% linewidth=0.88\linewidth
]
template <class T> vector<SecureMod>
convert(vector<T> v)
{
    vector<SecureMod> u;
    for (auto & e : v)
        u.push_back(SecureMod(e));
    return u;
}

template <int S> vector<SecureInt<S>>
indices(vector<SecureInt<S>> v)
{
  int size = v.size();
  vector<SecureInt<S>> idx;
  vector<vector<SecureInt<S>>> m(size);
  for (int i=0; i < size; i++)
  {
    for (int j=i+1; j < size; j++)
    {
      auto cond = v[i] > v[j];
      m[i].push_back(SecureInt<S>(cond));
      m[j].push_back(SecureInt<S>(!cond));
    }
    idx.push_back(sum(m[i]));
  }
  return idx;
}

template <int S> vector<SecureMod>
select(vector<SecureInt<S>> idx,
  vector<SecureMod> v)
{
  int size = v.size();
  vector<SecureMod> r;
  for (int i=0; i < size; i++)
  {
    vector<SecureMod> t;
    for (int j=0; j < size; j++ )
      t.push_back((i == idx[j]) * v[j]);
    r.push_back(sum(t));
  }
  return r;
}

template <int S> vector<SecureMod>
sort(vector<SecureInt<S>> & v)
{
  return select(indices(v), convert(v));
}


\end{lstlisting}
\end{minipage}
% \vspace{\lstbspace}
\end{figure}
